# Supplementary material for: Evaluating Transferable Emotion Expressions for Zoomorphic Social Robots using VR Prototyping
Source: arXiv:2410.15486 source file (2024-10-20)
Supplement: Supplementary file 1 [file ISMAR_Appendices.pdf]

**A DEMOGRAPHICS TABLE**

| Participant ID | Age | Gender | VR Exposure   | Robot Exposure | NARS |
|----------------|-----|--------|---------------|----------------|------|
| P1             | 21  | Woman  | Many times    | No             | 37   |
| P2             | 22  | Man    | Many times    | No             | 41   |
| P3             | 29  | Woman  | A few times   | Yes            | 31   |
| P4             | 23  | Woman  | A few times   | Maybe          | 28   |
| P5             | 25  | Man    | Never         | Yes            | 30   |
| P6             | 26  | Man    | Several times | Yes            | 29   |
| P7             | 30  | Woman  | Never         | No             | 37   |
| P8             | 26  | Man    | Many times    | No             | 47   |
| P9             | 23  | Woman  | Once or twice | No             | 40   |
| P10            | 25  | Woman  | Several times | No             | 37   |
| P11            | 21  | Woman  | A few times   | No             | 23   |
| P12            | 25  | Woman  | A few times   | No             | 26   |
| P13            | 23  | Man    | A few times   | Yes            | 15   |
| P14            | 23  | Man    | A few times   | No             | 33   |
| P15            | 29  | Woman  | Once or twice | No             | 29   |
| P16            | 37  | Woman  | A few times   | No             | 41   |
| P17            | 25  | Woman  | Never         | Yes            | 31   |
| P18            | 27  | Woman  | Never         | No             | 36   |
| P19            | 28  | Woman  | Once or twice | No             | 49   |
| P20            | 29  | Woman  | Once or twice | No             | 49   |
| P21            | 21  | Woman  | A few times   | No             | 41   |
| P22            | 32  | Woman  | Once or twice | No             | 41   |
| P23            | 23  | Woman  | Never         | Yes            | 39   |
| P24            | 24  | Woman  | Once or twice | No             | 42   |
| P25            | 23  | Man    | Many times    | No             | 38   |
| P26            | 40  | Man    | Many times    | No             | 38   |
| P27            | 30  | Man    | A few times   | No             | 37   |
| P28            | 24  | Man    | Many times    | Yes            | 32   |

Table 3. Table displaying the individual full demographic data taken for each of the 28 participants.

## B QUALITATIVE CODE-BOOKS SEPARATED BY QUESTION

| Category           | Codes        | Sub-Codes                                | #  |
|--------------------|--------------|------------------------------------------|----|
| Interpretability   | Clarity      |                                          | 25 |
|                    |              | Clarity - TTS                            | 2  |
|                    |              | Clarity - Emoji                          | 3  |
|                    |              | Clarity - Face                           | 5  |
|                    |              | Clarity - Text                           | 2  |
|                    |              | Clarity - Tail                           | 1  |
|                    | Unclear      |                                          | 21 |
|                    |              | Unclear - TTS                            | 1  |
|                    |              | Unclear - Text                           | 2  |
|                    |              | Unclear - Sound                          | 4  |
|                    |              | Unclear - Light                          | 9  |
|                    |              | Unclear - Tail                           | 3  |
| Familiar           | Familiar     |                                          | 19 |
|                    |              | Familiarity/Understandable - Emoji       | 4  |
|                    |              | Familiarity/Understandable - Face        | 4  |
|                    |              | Familiarity/Understandable - Tail        | 3  |
|                    |              | Familiarity/Understandable - Sound       | 1  |
|                    |              | Association - Light/Sound                | 2  |
|                    | Unfamiliar   |                                          | 10 |
|                    |              | Learning Needed                          | 3  |
|                    |              | Unfamiliarity/Not Understandable - Tail  | 1  |
|                    |              | Unfamiliarity/Not Understandable - Light | 4  |
|                    |              | Unfamiliarity/Not Understandable - Sound | 2  |
| Emotional Response | Emotive      |                                          | 20 |
|                    |              | Emotive - Sound                          | 3  |
|                    |              | Emotive - Tail                           | 3  |
|                    |              | Emotive - Face                           | 5  |
|                    |              | Emotive - Light                          | 2  |
|                    |              | Emotive - Emoji                          | 1  |
|                    | Unemotive    |                                          | 19 |
|                    |              | Unemotive - TTS                          | 5  |
|                    |              | Unemotive - Text                         | 6  |
|                    |              | Unemotive - Light                        | 2  |
|                    |              | Unemotive - Sound                        | 1  |
|                    |              | Discomfort - TTS                         | 1  |
| Amusing/Cute       | Amusing/Cute |                                          | 5  |
|                    |              | Amusing/Cute - Face                      | 3  |
|                    |              | Amusing/Cute - Sound                     | 1  |
| Natural/Lifelike   | Natural      |                                          | 29 |
|                    |              | Natural/Lifelike - Face                  | 8  |
|                    |              | Natural/Lifelike - TTS                   | 1  |
|                    |              | Natural/Lifelike - Sound                 | 3  |
|                    |              | Natural/Lifelike - Emoji                 | 2  |
|                    |              | Natural/Lifelike - Tail                  | 4  |
|                    | Unnatural    |                                          | 7  |
|                    |              | Unnatural/Unlifelike - Text              | 1  |
|                    |              | Unnatural/Unlifelike - TTS               | 4  |
|                    |              | Unnatural/Unlifelike - Light             | 2  |

Table 4. Table displaying the qualitative code-book categories, codes and sub-codes applied to data from the **Modality Rankings** free-text question.

| Category               | Codes                                            | Sub-Codes                     | #  |
|------------------------|--------------------------------------------------|-------------------------------|----|
| No Frame of Reference  | Interaction Expectations - No Basis              |                               | 3  |
|                        |                                                  | Anthropomorphised Qoobo       | 1  |
|                        | Communication Wall                               |                               | 3  |
|                        |                                                  | Impact - Misinterpretation    | 2  |
|                        |                                                  | Unclear                       | 1  |
| Pet Frame of Reference | Expectations/Perceptions Based on Pet Experience |                               | 15 |
|                        |                                                  | Natural Cues seen as Lifelike | 13 |
|                        |                                                  | Natural/Lifelike              | 3  |
|                        |                                                  | Natural/Lifelike - Tail       | 7  |
|                        |                                                  | Natural/Lifelike - Face       | 1  |
|                        |                                                  | Natural/Lifelike - Fur        | 2  |
|                        | Emotional Connection                             |                               | 8  |
|                        |                                                  | Emotional Connection          | 5  |
|                        |                                                  | Emotional Connection - Tail   | 3  |
|                        | Increased Expectation                            |                               | 3  |
|                        |                                                  | Unemotive / Lack of Movement  | 1  |
|                        |                                                  | Robot Expression Too Simple   | 1  |
| Experience             | Cognitive Dissonance                             |                               | 1  |
|                        | Experience                                       |                               | 37 |
|                        |                                                  | Experience - Low              | 3  |
|                        |                                                  | Experience Varied             | 3  |
|                        |                                                  | Experience - Yes - Cat        | 9  |
|                        |                                                  | Experience - Yes              | 12 |
|                        |                                                  | Experience - Yes - Dog        | 7  |
|                        |                                                  | Experience - No               | 5  |
| Impact of Experience   | Impact of Experience                             |                               | 18 |
|                        |                                                  | Impact - Partial              | 5  |
|                        |                                                  | Impact - Positive             | 2  |
|                        |                                                  | Impact - Yes                  | 9  |
|                        |                                                  | Impact - No                   | 2  |

Table 5. Table displaying the qualitative code-book categories, codes and sub-codes applied to data from the **Animal Experience** free-text question.

Table displaying the qualitative code-book categories, codes and sub-codes applied to data from the **Animal Experience** free-text question.

| Category                     | Codes | Sub-Codes                                   | #  |
|------------------------------|-------|---------------------------------------------|----|
| Natural                      |       |                                             | 25 |
|                              |       | Evocative/Lifelike                          | 16 |
|                              |       | Naturalistic Modes More Affective           | 9  |
|                              |       | Evocative/Lifelike - Face                   | 2  |
|                              |       | Instinctive understand                      | 2  |
|                              |       | Impact of Natural Modes                     | 6  |
|                              |       | Natural Modes Lack Clarity                  | 3  |
|                              |       | Robot Could be Scary if Acts Unnatural      | 1  |
|                              |       | Natural modes improved safety / familiarity | 1  |
|                              |       | Fear/Anxiety about Misintepretation         | 1  |
| Technical                    |       |                                             | 20 |
|                              |       | Tech Modes Add Clarity                      | 9  |
|                              |       | Technological Modes Add Clarity - Speech    | 2  |
|                              |       | Technological Modes Add Clarity - Text      | 3  |
|                              |       | Technological Modes Add Clarity - Light     | 1  |
|                              |       | Technological Modes Add Clarity - Emoji     | 2  |
|                              |       | Reduced Social/Emotional Impact             | 8  |
|                              |       | Technological Modes Less Affective          | 3  |
|                              |       | Unevocative/Not Realistic                   | 4  |
|                              |       | Technological Modes Reduced Prescence       | 1  |
|                              |       | Tech Unconstrained                          | 3  |
|                              |       | Adding Technology Adds Fun Function         | 2  |
|                              |       | Amusing/Cute - Emoji                        | 1  |
| General Modality Preferences |       |                                             | 47 |
|                              |       | Preference - Neither                        | 1  |
|                              |       | Preference - Combination                    | 9  |
|                              |       | Preference - Either                         | 1  |
|                              |       | Preference - Naturalistic                   | 19 |
|                              |       | Preference - Technological                  | 1  |
|                              |       | Allow users to customise                    | 1  |
|                              |       | Familiarity                                 | 10 |
|                              |       | Differences in Modality Classification      | 5  |
|                              |       | Disagree with Classification                | 1  |
|                              |       | Disagree with Classification - Sound        | 1  |
|                              |       | Disagree with Classification - Light        | 1  |
|                              |       | Mode felt more natural than technological   | 1  |
|                              |       | Mode felt more technological than natural   | 1  |

Table 6. Table displaying the qualitative code-book categories, codes and sub-codes applied to data from the **Natural versus Technological Modes** free-text question.

| Category                          | Codes | Sub-Codes                                          | #   |
|-----------------------------------|-------|----------------------------------------------------|-----|
| Grounded in Natural and Evocative |       |                                                    | 129 |
|                                   |       | Emotive                                            | 70  |
|                                   |       | Sad Sound Evocative/Fitting                        | 12  |
|                                   |       | Sadness can be expressed too intensely             | 1   |
|                                   |       | Amusing/Cute - Tail                                | 2   |
|                                   |       | Amusing/Cute - Emoji                               | 2   |
|                                   |       | Amusing/Cute - Face                                | 1   |
|                                   |       | Amusing/Cute - Light                               | 3   |
|                                   |       | Amusing/Cute - Text                                | 1   |
|                                   |       | Emotive - Tail                                     | 11  |
|                                   |       | Emotive - Light                                    | 7   |
|                                   |       | Emotive - Sound                                    | 5   |
|                                   |       | Emotive - Emoji                                    | 5   |
|                                   |       | Emotive - Face                                     | 14  |
|                                   |       | Emotive/Emotional Connection                       | 6   |
|                                   |       | Unemotive                                          | 5   |
|                                   |       | Unemotive - Tail                                   | 1   |
|                                   |       | Unemotive - Text                                   | 1   |
|                                   |       | Unemotive - Emoji                                  | 1   |
|                                   |       | Unemotive - Face                                   | 1   |
|                                   |       | Unemotive - Sound                                  | 1   |
|                                   |       | Natural/Lifelike                                   | 46  |
|                                   |       | Natural Modes More Affective                       | 7   |
|                                   |       | Natural modes improved safety / familiarity        | 1   |
|                                   |       | Anthromorphising Robot                             | 1   |
|                                   |       | Natural/Lifelike - Tail                            | 18  |
|                                   |       | Natural/Lifelike - Sound                           | 5   |
|                                   |       | Natural/Lifelike - Face                            | 12  |
|                                   |       | Natural/Lifelike - Light                           | 2   |
|                                   |       | Unnatural/Unlifelike                               | 8   |
|                                   |       | Unnatural/Unlifelike - Light                       | 3   |
|                                   |       | Unnatural/Unlifelike - Text                        | 1   |
|                                   |       | Unnatural/Unlifelike - Sound                       | 2   |
|                                   |       | Unnatural/Unlifelike - Emoji                       | 1   |
|                                   |       | Unnatural/Unlifelike - TTS                         | 1   |
| Need for Interpretability         |       |                                                    | 85  |
|                                   |       | Social Inference                                   | 4   |
|                                   |       | Comfort in Clarity                                 | 1   |
|                                   |       | Interpretability Challenges                        | 22  |
|                                   |       | Preferred Alternative Mode Option                  | 11  |
|                                   |       | Emotion-specific Modes                             | 6   |
|                                   |       | Differences in Colour Meaning/Preference           | 5   |
|                                   |       | Familiarity/Understandable                         | 19  |
|                                   |       | Interactions Expectation - Based on Pet            | 1   |
|                                   |       | Familiarity/Understandable - Text                  | 1   |
|                                   |       | Familiarity/Understandable - Face                  | 6   |
|                                   |       | Familiarity/Understandable - Tail                  | 6   |
|                                   |       | Familiarity/Understandable - Emoji                 | 2   |
|                                   |       | Familiarity/Understandable - Light                 | 2   |
|                                   |       | Unfamiliarity/Not Understandable - Tail            | 1   |
|                                   |       | Clarity                                            | 40  |
|                                   |       | Clarity - Emoji                                    | 10  |
|                                   |       | Clarity - Face                                     | 10  |
|                                   |       | Clarity - Tail                                     | 4   |
|                                   |       | Clarity - Light                                    | 4   |
|                                   |       | Clarity - Text                                     | 6   |
|                                   |       | Clarity - Sound                                    | 2   |
|                                   |       | Unclear                                            | 4   |
|                                   |       | Unclear - Sound                                    | 2   |
|                                   |       | Unclear - Tail                                     | 2   |
| Rationale for Multimodal          |       |                                                    | 47  |
|                                   |       | Adding Modes Adds Clarity                          | 18  |
|                                   |       | Technological Modes Add Clarity                    | 10  |
|                                   |       | Use All Senses                                     | 4   |
|                                   |       | Emoji more Clear and Emotive than other Tech Modes | 2   |
|                                   |       | Adding Technology Adds Fun/Function                | 2   |
|                                   |       | Amplify/Compliment Emotion                         | 29  |
|                                   |       | Amplifies Emotion                                  | 9   |
|                                   |       | Complimentary Modes                                | 12  |
|                                   |       | Diffusing the Emotion into the Room                | 7   |
|                                   |       | Text could facilitate deeper communication         | 1   |

Table 7. Table displaying the qualitative code-book categories, codes and sub-codes applied to data from the **Prototyping Rationale** interview.

## C POST STUDY SURVEY AND POST-PROTOTYPING INTERVIEW QUESTIONS

Note: while these questions were initially delivered either via a website interface or verbally, all are presented in native text here for accessibility.

### C.1 Post-Session Survey

1.a. Looking back at the 7 modes that VR Qoobo used to show emotion in this experiment, please rank them from most to least preferred.

*(Participants dragged these items into their preferred order in the web interface.)*

- Facial Expressions
- Tail Movement
- Sounds
- Emoji Thought Bubbles
- Floating Text
- Spoken Text
- Coloured Light

1.b. Why did you prefer the modes you ranked higher, or dislike the modes you ranked lower?

*(Participants were given a mandatory free-text field to answer this question.)*

2.a. Do you have any prior personal experience with domesticated animals (such as pets or farm animals)?

*(Participants were given a mandatory free-text field to answer this question.)*

2.b. If so, do you think this experience impacted your impressions of the robot and its emotional expression? How?

*(Participants were given a mandatory free-text field to answer this question.)*

3. The modes of emotional expression seen in this experiment could be divided into two categories. Naturalistic modes are already seen in real animals, such as facial expressions, tail movement and sound. Technological modes, like floating text, speech, colours or emoji, are not available to animals and but can be facilitated by robots or virtual reality. Did you prefer either approach more? Why? *(Participants were given a mandatory free-text field to answer this question.)*

### C.2 Post-Prototyping Interview

*(Following consent to record the participant's voice.)*

Researcher: "Could you walk me through the design you chose to express emotions and why you chose those elements?"

*(wait for response)*

If answer is short ask follow up questions: "Thanks. Can you explain this a bit more?", "Interesting. Can you expand on this thought?"

If only one, or neither specific emotion is discussed, ask ask follow up question: "Thanks. Could you now walk me through why you specifically chose <modalities> for <emotion>?"
